# Supplementary material for: Synthesizing Robust Walking Gaits via Discrete-Time Barrier Functions with Application to Multi-Contact Exoskeleton Locomotion
Source: arXiv:2310.06169 source file (2024-03-13)
Supplement: Supplementary file 1 [file Appendix.tex]

\newpage
\section{Appendix}

\subsection{Deriving the continuous-time and discrete-time dynamics for robotic legged systems}
For robotic systems, the continuous-time dynamics can be derived using the Euler-Lagrange equations, resulting in the expression:
\begin{align}
    D(q_e)\ddot{q_e} + H(q_e,\dot{q_e}) = Bu, 
\end{align}
with $D: \mathcal{Q} \to \R^{n \times n}$ denoting the inertia matrix, $H: \mathsf{T}\mathcal{Q} \to \R^n$ denoting the drift vector, and $B \in \R^{n \times m}$ denoting the actuation matrix labeling the actuated states of the system for some input $u \in \mathcal{U} \subset \R^m$. Using this representation, the full continuous-time dynamics are of the form:
\begin{align}
    \dot x = \underbrace{\begin{bmatrix}
        \dot q_e \\ -D(q_e)^{-1}H(q_e, \dot q_e) 
    \end{bmatrix}}_{f(x)} + \underbrace{\begin{bmatrix}0\\D(q_e)^{-1}B\end{bmatrix}}_{g(x)}u.
\end{align}

Concurrently, a common method for describing the discrete-time dynamics that occurs at impact is through the momentum transfer equation \cite{hurmuzlu1994rigid}. Specifically, as the system flows into the guard, $n_c \in \mathbb{N}$ holonomic constraints $c:\mathcal{Q}\to \R^{n_c}$ are enforced in the continuous domain succeeding the impact event, and the system undergoes a discrete jump in the state as captured by the momentum transfer equation \cite{hurmuzlu1994rigid}:
\begin{align}
    D(q_e^-)(\dot q_e^+ - \dot q_e^-) = J_c(q_e^-)^\top \delta F
\end{align}
where $q_e^-, q_e^+ \in \mathcal{Q}$, and $\dot q_e^-, \dot q_e^+\in\R^n$ represent the robot configuration and velocity just before and after impact, respectively, $\delta F \in \R^{n_c}$ is the impulse force of the impact event, and $J_c:\mathcal{Q}\to \R^{n_c\times n}$ is the Jacobian of the holonomic constraints. This can equivalently be represented via its derivative, $J_c(q_e^-) \dot q_e^+ = 0$. With this, we can rewrite the impact equation \cite{glocker1992dynamical} as:
\begin{align}
    \begin{bmatrix}
        D(q_e^-) & -J_c(q_e^-)^\top \\ J_c(q_e^-) & 0
    \end{bmatrix}
    \begin{bmatrix}
        \dot{q}_e^+ \\ \delta F
    \end{bmatrix} = 
    \begin{bmatrix}
        D(q_e^-)\dot{q}_e^{-} \\ 0
    \end{bmatrix}. \label{eq: impactrelation}
\end{align}
Noting that the configuration is continuous through impact, solving for $\dot q_e^+$ in \eqref{eq: impactrelation} allows us to define the \textit{reset map} $\Delta: \S \to \S$, i.e. the map describing the discrete event at footstrike \cite{grizzle2014models}, as:
\begin{align}
    \small
    \Delta(x^-) := \begin{bmatrix}
        \Delta_{q_e} \\ \Delta_{\dot{q}_e}
    \end{bmatrix} = 
    \begin{bmatrix}
        Rq_e^- \\ R(-D^{-1}J_c^{\top}(J_c D^{-1}J_c^{\top})^{-1} J_c + I)\dot{q}_e^-    
    \end{bmatrix}
    \label{eq: reset}
\end{align}
where the dependence of $D$ and $J_c$ on $q_e^-$ is suppressed and $R \in \R^{n \times n}$ denotes the relabeling matrix which is used to maintain state consistency between domains.

\subsection{HZD Method for Gait Generation}
Consider a robotic system with coordinates $q \in \mathcal{Q}\subset\mathbb{R}^n$ and system state $x=(q,\dot q)\in \mathsf T\mathcal{Q}$, where $\mathsf T\mathcal{Q}$ denotes the tangent bundle of the configuration manifold $\mathcal{Q}$. In the case of the Atalante lower-body exoskeleton, \red{...}.

The hybrid zero dynamics (HZD) method presented by \cite{westervelt2003hybrid} is a mathematical framework that synthesizes feedback controllers to systematically achieve exponentially stable hybrid periodic orbits. In short, this is accomplished by selecting the desired behavior of the system outputs during the continuous dynamics such that the resulting closed-loop system is rendered invariant through impacts. 

 In summary, the method constructs a periodic orbit $\O$ by defining the controllable outputs (termed virtual constraints) of the continuous-time system, and driving these outputs to zero using an input-output linearizing controller. The system then evolves on the zero dynamics surface: 
\begin{align}
    \Z = \{x \in \X \mid y(x) = 0, ~L_fy(x) = 0 \}.
\end{align}
with $y: \X \to \in \R^k$ denoting the virtual constraints. 
% Note that generally, hybrid zero dynamics are defined analogously to zero dynamics \cite{isidori1985nonlinear} as: the largest internal dynamics compatible with the output being identically zero.

Lastly, per Def. 1 of \cite{westervelt2003hybrid}, assuming impact-invariance of the zero dynamics surface ($\Delta(\S \cap \Z) \subset \Z$), then the \textit{hybrid zero dynamics} of the system are defined as:
\begin{numcases}{}
    \dot{z} = \omega(\eta,z) & $z \not\in \S \cap \Z$\\
    z^+ = \Delta_{\Z}(z^-) & $z^- \in \S \cap \Z$,
\end{numcases}
where $\dot{z} = \omega(\eta,z)$ is the continuous dynamics of the uncontrollable states $z \in \R^{n-k}$ (termed the zero dynamics). Note that the impact-invariance assumption is required to construct periodic orbits along which the output $y(x)$ is identically zero.

The Hybrid Zero Dynamics method of gait generation synthesizes nominal walking gaits as periodic orbits that remain invariant through pre-defined contact sequences. The most common domain graphs used are illustrated in Fig. ?: a single-domain, single-edge, structure used to describe flat-foot locomotion, and a two-domain, two-edge structure used to describe foot-rolling locomotion. Note that it is also possible to describe multicontact locomotion using three or four domains \cite{huihua, gehlhar, reher}.

Once a contact sequence is specified, the dynamics associated with the walking behavior are described as a hybrid system, continuous-time domains and discrete-time impact events. The admissible domain on which the system evolves is denoted $\mathcal{D} \subset \mathsf T\mathcal{Q}$. This set captures the admissible set of states for the system (i.e. the set of states with swing foot above the floor, which respecting joint limits, etc). One method of deriving the continuous-time dynamics of the system is using the Euler-Lagrange equations, which results in the expression:
\begin{align}
    \dot x = \underbrace{\begin{bmatrix}
        \dot q \\ -D(q)^{-1}H(q, \dot q) 
    \end{bmatrix}}_{f(x)} + \underbrace{\begin{bmatrix}0\\D(q)^{-1}B\end{bmatrix}}_{g(x)}u.
\end{align}
where $D:\mathcal{Q}\to \mathbb{R}^{n\times n}$ is the mass-inertia matrix, $H:\mathsf T\mathcal{Q}\to \mathbb{R}^n$ contains the Coriolis and gravity terms, $B\in\mathbb{R}^{n\times m}$ is the actuation matrix, and $u \in \R^m$ is the control input. 

Next, we define the \textit{guard}, the set of states where a discrete impact event will occur. Letting $p_{sw}^z:\mathcal{Q}\to\mathbb{R}$ return the vertical position of the swing foot, the guard for the systems investigated in this work (assuming a known and constant ground height of zero) is defined as: \begin{align}
    \mathcal{S} = \{x\in \mathcal{D} ~|~ p^z_{sw}(q) = 0,~ \dot p^z_{sw}(x) < 0\},
\end{align}
or the set of states when the swing foot strikes the ground with a negative velocity. As the system flows into the guard, $n_c \in \mathbb{N}$ holonomic constraints $c:\mathcal{Q}\to \R^{n_c}$ are enforced in the continuous domain succeeding the impact event, and the system undergoes a discrete jump in the state as captured by the momentum transfer equation \cite{hurmuzlu1994rigid}:
\begin{align}
    D(q^-)(\dot q^+ - \dot q^-) = J_c(q^-)^\top \delta F
\end{align}
where $q^-, q^+ \in \mathcal{Q}$, and $\dot q^-, \dot q^+\in\R^n$ represent the robot configuration and velocity just before and after impact, respectively, $\delta F \in \R^{n_c}$ is the impulse force of the impact event, and $J_c:\mathcal{Q}\to \R^{n_c\times n}$ is the Jacobian of the holonomic constraints.

% This can equivalently b represented via its derivative, J(q^+) \dot q^+ = 0

Enforcing the holonomic constraints through impacts can equivalently be represented as $J_c(q^-)\dot q^+ = 0$. With this, we can rewrite the impact equation \cite{glocker1992dynamical} as:
\begin{align}
    \begin{bmatrix}
        D(q^-) & -J_c(q^-)^\top \\ J_c(q^-) & 0
    \end{bmatrix}
    \begin{bmatrix}
        \dot{q}^+ \\ \delta F
    \end{bmatrix} = 
    \begin{bmatrix}
        D(q^-)\dot{q}^{-} \\ 0
    \end{bmatrix}. \label{eq: impactrelation}
\end{align}
Noting that the configuration is continuous through impact, solving for $\dot q^+$ in \eqref{eq: impactrelation} allows us to define the \textit{reset map} $\Delta: \mathcal{S} \to \mathcal{D}$, i.e. the map describing the discrete event at footstrike \cite{grizzle2014models}, as:
\begin{align}
    \small
    \Delta(x^-) := \begin{bmatrix}
        \Delta_{q} \\ \Delta_{\dot{q}}
    \end{bmatrix} = 
    \begin{bmatrix}
        Rq^- \\ R(-D^{-1}J_c^{\top}(J_c D^{-1}J_c^{\top})^{-1} J_c + I)\dot{q}^-    
    \end{bmatrix}
    \label{eq: reset}
\end{align}
where the dependence of $D$ and $J_c$ on $q^-$ is suppressed and $R \in \R^{n \times n}$ denotes the relabeling matrix which is used to maintain state consistency between domains. We are now fully equipped to define the hybrid system of walking as:
\begin{align}
\mathcal{H}\mathcal{C} = 
    \begin{cases}
        \dot{x} = f(x) + g(x)u, & x \in \mathcal{D} \backslash\mathcal{S}, \\
        x^+ = \Delta (x^-), & x \in \mathcal{S}.
    \end{cases}
\end{align}
Note that hybrid systems with a more diverse collection of contact sequences can be modeled via the same framework \cite{sinnet20092d, zhao2017multi, reher2020algorithmic}, at the cost of introducing a directed graph describing how the continuous and discrete domains are related -- this is omitted in this work for the sake of simplicity.

\newsec{Trajectory Optimization}
The hybrid zero dynamics (HZD) method of gait generation leverages trajectory optimization in the context of the aforementioned hybrid control system to synthesize provably stable walking trajectories (gaits), encoded as nontrivial limit cycles \cite{grizzle20103d}.  
% One of the main benefits of this method is that it is able to directly account for the discrete impact events.

 We begin by defining a collection of $k \in \mathbb{N}$ \textit{outputs} or \textit{virtual constraints} $y_{\alpha}: \mathcal{Q} \to \R^k$ which we would like to converge to zero. These virtual constraints encode the desired behavior of the system via:
\begin{align}
    y_{\alpha}(q) = y^a(q) - y^d_\alpha(\tau(q)),
\end{align}
where $y^a: \mathcal{Q} \to \R^k$ represents the actual (measured) outputs of the system, $y^d_\alpha: \R \to \R^k$ represents the desired outputs commonly parameterized via a $p^{\text{th}}$-order B\'ezier polynomial with B\'ezier coefficients $\alpha \in \R^{k \times p+1}$, and $\tau: \mathcal{Q} \to [0,1]$ is a monotonically increasing variable over the gait cycle, termed a \textit{phasing variable}. The HZD framework reduces the stability analysis of the system $\mathcal{H}\mathcal{C}$ to a lower-dimensional manifold, the \textit{zero dynamics surface}:
\begin{align}
    \mathcal{Z}_{\alpha} := \{ x \in \mathcal{D} ~|~ y_{\alpha}(q) = 0, \dot{y}_{\alpha}(x) = 0\},
\end{align}
%
% where $y: \mathcal{Q} \to \R^m$ denotes the \textit{outputs} or \textit{virtual constraints}. These virtual constraints encode the desired behavior of the system via:
% \begin{align}
    % y(q,\alpha) = y^a(q) - y^d(\tau(q),\alpha),
% \end{align}
% with $y^a: \mathcal{Q} \to \R^m$ describing the actual (measured) outputs of the system, and $y^d: \R \times \mathcal{Q} \to \R^m$ describing the desired outputs. It is common to parameterize $y^d$ as a $b^{\text{th}}$-order B\'ezier polynomial defined using a phasing variable $\tau: \mathcal{Q} \to \R$ and B\'ezier coefficients $\alpha \in \R^{m \times b+1}$. 
%
% Driving the outputs to zero using a stabilizing controller $u^*: \mathcal{D} \to \R^m$, for example a feedback linearizing or control Lyapunov function based controller, results in a closed loop dynamical system: $\dot{x} = f_{cl}(x) := f(x) + g(x)u^*(x)$. 
%
% The virtual constraints are driven to zero using a stabilizing controller $u^*: \mathcal{D} \to \R^m$. This results in a closed loop dynamical system: $\dot{x} = f_{cl}(x) := f(x) + g(x)u^*(x)$. 
%
which can be rendered impact-invariant by enforcing the \textit{HZD condition}:
\begin{align}
    \Delta(\mathcal{S} \cap \mathcal{Z}_{\alpha}) \subset \mathcal{Z}_{\alpha}. \label{eq: HZDcondition}
\end{align}

Driving the outputs to zero using a stabilizing controller $u^*: \mathcal{D} \to \R^m$, for example a feedback linearizing or control Lyapunov function based controller, results in a closed loop dynamical system: $\dot{x} = f_{cl}(x) := f(x) + g(x)u^*(x)$. 
This stabilizing controller, paired with the HZD condition and an orbit which is stable on the zero dynamics surface renders the closed loop hybrid dynamical system stable. 
Importantly, the stability of the zero dynamics on $\mathcal{Z}_{\alpha}$ can be shaped through the choice of outputs and B\'ezier coefficients $\alpha$. Therefore, an optimization problem is constructed to synthesize trajectories with desired outputs such that \eqref{eq: HZDcondition} is enforced. This optimization problem takes the form:
\begin{align}
    \{\alpha^*, X^*\} &= \argmin_{\alpha, X} ~\Phi(X) \label{eq: NLP}\\
    \text{s.t.} \quad &\dot{x} = f_{cl}(x) \tag{Closed-loop Dynamics} \\
    &\Delta(\mathcal{S} \cap \mathcal{Z}_{\alpha}) \subset \mathcal{Z}_{\alpha} \tag{HZD Condition} \\
    &X_{\text{min}} \preceq X \preceq X_{\text{max}} \tag{Decision Variables} \\
    &a_{\text{min}} \preceq a(X) \preceq a_{\text{max}} \tag{Physical Constraints}
\end{align}
In this NLP, $X = (x_0, \dots, x_N, T) \in \mathcal{X} $ is the collection of all decision variables with $x_i \in \R^{2n}$ being the state at the $i^{\text{th}}$ collocation point and $T \in \R$ the total duration, $\Phi: \mathcal{X} \to \R$ denotes the cost function (such as torque-squared or mechanical cost of transport \cite{reher2020algorithmic}), and $a(X)$ is the set of physical constraints which includes holonomic constraints, workspace limits, power limits, etc. The solution of \eqref{eq: NLP} is a limit cycle which encodes stable walking, described by some static set of B\'ezier coefficients $\alpha^* \in \R^{k \times p+1}$.

% \red{maybe talk about constraint tuning here?}
